# Supplementary material for: Fast Benchmarking of Asynchronous Multi-Fidelity Optimization on Zero-Cost Benchmarks
Source: arXiv:2403.01888 source file (2024-08-19)
Supplement: Supplementary file 1 [file wrapper-args.tex]

\section{Wrapper Object (\texttt{ObjectiveFuncWrapper})}
\label{appx:wrapper:section}
In this section, we describe more details on our wrapper.

\subsection{Arguments}
\label{appx:wrapper-args:section}
The arguments of \texttt{ObjectiveFuncWrapper} object are as follows:
\begin{itemize}
  \vspace{-1.5mm}
  \item \texttt{obj\_func}: the objective function that takes (\texttt{eval\_config}, \texttt{fidels}, \texttt{seed}, \texttt{**data\_to\_scatter}) as arguments and returns $f(\xv|\av)$ and $\tau(\xv|\av)$ where \texttt{eval\_config} is \texttt{dict[str, Any]},
  \vspace{-1.5mm}
  \item \texttt{launch\_multiple\_wrappers\_from\_user\_side (bool)}: whether to instantiate multiple wrappers from userside (e.g. NePS that uses file-based synchronization) or not (e.g. DEHB that uses multiprocessing that spawns subprocesses),
  \vspace{-1.5mm}
  \item \texttt{ask\_and\_tell (bool)}:
  whether to use simulator for ask-and-tell interface (\texttt{True}) or not,
  \vspace{-1.5mm}
  \item \texttt{save\_dir\_name (str | None)}: the results and the required information will be stored in \texttt{mfhpo-simulator-info/<save\_dir\_name>/},
  \vspace{-1.5mm}
  \item \texttt{n\_workers (int)}: the number of parallel workers $P$,
  \vspace{-1.5mm}
  \item \texttt{n\_evals (int)}: the number of evaluations to get,
  \vspace{-1.5mm}
  \item \texttt{n\_actual\_evals\_in\_opt (int)}: the number of HP configurations to be evaluated in an optimizer which is used only for checking if no hang happens (should take \texttt{n\_evals + n\_workers}),
  \vspace{-1.5mm}
  \item \texttt{continual\_max\_fidel (int | None)}:  when users would like to restart each evaluation from intermediate states, the maximum fidelity value for the target fidelity must be provided.
  Note that the restart is allowed only if there is only one fidelity parameter.
  If \texttt{None}, no restart happens as in Line~\ref{main:methods:line:continual-eval} of Algorithm~\ref{main:methods:alg:automatic-job-alloc-wrapper},
  \vspace{-1.5mm}
  \item \texttt{runtime\_key (str)}: the key of the runtime in the returned value of \texttt{obj\_func},
  \vspace{-1.5mm}
  \item \texttt{obj\_keys (list[str])}: the keys of the objective and constraint names in the returned value of \texttt{obj\_func} and the values of the specified keys will be stored in the result file,
  \vspace{-1.5mm}
  \item \texttt{fidel\_keys (list[str] | None)}: the keys of the fidelity parameters in input \texttt{fidels},
  \vspace{-1.5mm}
  \item \texttt{seed (int | None)}: the random seed to be used in the wrapper,
  \vspace{-1.5mm}
  \item \texttt{max\_waiting\_time (float)}: the maximum waiting time for each worker and if each worker did not get any update for this amount of time, it will return \texttt{inf},
  \vspace{-1.5mm}
  \item \texttt{store\_config (bool)}: whether to store configurations, fidelities, and seed used for each evaluation, and
  \vspace{-1.5mm}
  \item \texttt{check\_interval\_time (float)}: how often each worker should check whether a new job can be assigned to it.
  \vspace{-1.5mm}
\end{itemize}
Note that \texttt{data\_to\_scatter} is especially important when an optimizer uses multiprocessing packages such as \texttt{dask} or \texttt{multiprocessing}, which deserialize \texttt{obj\_func} every time we call.
By passing large-size data via \texttt{data\_to\_scatter}, the time for (de)serialization will be negligible if optimizers use \texttt{dask.scatter} or something similar internally.
We kindly ask readers to check any updates to the arguments at
\ifunderreview
\url{https://anonymous.4open.science/r/mfhpo-simulator-3C81/README.md}.
\else
\url{https://github.com/nabenabe0928/mfhpo-simulator/}.
\fi

\subsection{Wrapper for Ask-and-Tell Interface}
\label{appx:wrapper-ask-and-tell:section}
When optimizers take ask-and-tell interface, simulations can be run on a single worker while preserving the results, and hence simulations can be further accelerated.
Note that the bottleneck of simulations is the waiting time due to the communication among each worker and simulations on a single worker can address this problem.
The benefits of this option are (1) faster, (2) memory-efficient, and (3) stable.
On the other hand, the downsides are that (1) this option forces optimizers to have the ask-and-tell interface and (2) simulations may fail to precisely consider a bottleneck caused by parallel execution of expensive optimizers.
For more details, see \url{https://github.com/nabenabe0928/mfhpo-simulator/}.
